# Supplementary material for: Observation of oscillating $g$-factor anisotropy arising from strong crystal lattice anisotropy in GaAs spin-3/2 hole quantum point contacts
Source: arXiv:2211.00253 ancillary file (2022-11-07)
Supplement: Supplementary file 1 [file SM___Observation_of_oscillating_g_factor_anisotropy_arising_from_strong_crystal_lattice_anisotropy_in_GaAs_spin_32_hole_quantum_point_contacts.pdf]

# Supplementary Material: Observation of oscillating $g$-factor anisotropy arising from strong crystal lattice anisotropy in GaAs spin-3/2 hole quantum point contacts

K. L. Hudson,[1,2] A. Srinivasan,[1,2] D. S. Miserev,[3] Q. Wang,[1,2] O. Klochan,[1,2] O. Sushkov,[2] I. Farrer,[4] D. A. Ritchie,[5] and A. R. Hamilton[1,2]

[1]*School of Physics, University of New South Wales*
[2]*ARC Centre of Excellence for Future Low-Energy Electronics Technologies (FLEET)*
[3]*University of Basel, Switzerland*
[4]*University of Sheffield, United Kingdom*
[5]*Cavendish Laboratory, Cambridge, United Kingdom*

## I. CALCULATING THE $g$-FACTOR

This section contains the $g$-factors measured for each 1D subband in each QPC, along with the source-drain bias measurements used to obtain the subband energy spacing and lever arms used to calculate the $g$-factors.

The $g$-factor for each subband was calculated from Zeeman spin-splitting measurements using the following

$$\begin{aligned} \Delta E_Z &= g\mu_B B \\ &= e\frac{\partial V_{dc}}{\partial V_{SG}} \times \Delta V_{SG}(B) \\ &= e\alpha(V_{SG}) \times \Delta V_{SG}(B) \end{aligned} \tag{S1}$$

where $E_Z$ is the Zeeman energy, $V_{SD}$ is the source-drain bias, $V_{SG}$ the split-gate voltage and $\alpha(V_{SG})$ is the lever arm factor used to convert gate voltage to energy.

The extracted in-plane $g$-factors $g_\parallel$, for $\boldsymbol{B} \parallel \boldsymbol{I}$, and $g_\perp$, for $\boldsymbol{B} \perp \boldsymbol{I}$, $\boldsymbol{I}$ is the current direction though a QPC, are shown in **Fig. S1** and tabulated in **Table S1** for $n \geq 2$ 1D subbands in each QPC. Measured $g$-factors show no systematic dependence on the subband number $n$ within the error bars. This is consistent with the electrostatic calculations performed in Ref. [2] where the $g$-factors quickly saturate to a fixed value at subband numbers $n \geq 2$. This allows us to calculate the subband average of the $g$-factors, see **Table S1** and **Fig. 4** in the main text. Extraction of the $g$-factors for the first subband is obstructed by "0.7 anomaly" dwelling on the Coulomb interaction effects in the QPC channel [4].

Figure S2. is the grey-scale source-drain bias maps for each QPC, where the quantity of dc bias $V_{dc}$ applied to find subband crossings is used to find the 1D subband energy spacings $\Delta E_{n,n+1}$ and the factor $\alpha(V_{SG})$ (shown in Figure S3) used to convert gate voltage $V_{SG}$ to Zeeman spin splitting energy $\Delta E_Z$ in order to calculate $g$ in equation (S1).

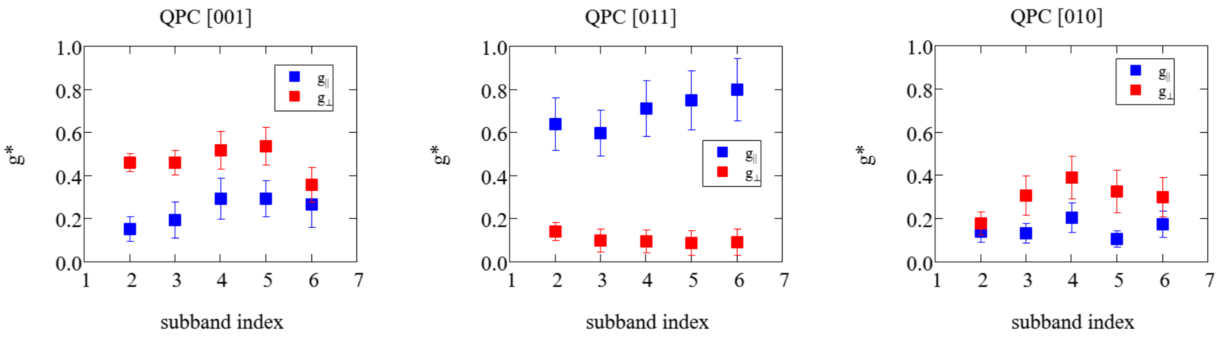


FIGURE S1: Measured $g$-factors for each subband index for (a) QPC [001], (b) QPC [011], and (c) QPC [010]. The $g$-factors are averaged over subbands 2-5 in order to compare the anisotropy in the main text.

| **Subband** | **QPC [001]** | | **QPC [011]** | | **QPC [010]** | |
|---|---|---|---|---|---|---|
| | $g_{\parallel}$ | $g_{\perp}$ | $g_{\parallel}$ | $g_{\perp}$ | $g_{\parallel}$ | $g_{\perp}$ |
| **2** | $0.153 \pm 0.057$ | $0.456 \pm 0.043$ | $0.639 \pm 0.121$ | $0.142 \pm 0.064$ | $0.140 \pm 0.049$ | $0.177 \pm 0.053$ |
| **3** | $0.192 \pm 0.087$ | $0.459 \pm 0.058$ | $0.595 \pm 0.107$ | $0.099 \pm 0.054$ | $0.134 \pm 0.047$ | $0.308 \pm 0.092$ |
| **4** | $0.293 \pm 0.096$ | $0.519 \pm 0.088$ | $0.710 \pm 0.128$ | $0.095 \pm 0.052$ | $0.203 \pm 0.071$ | $0.389 \pm 0.117$ |
| **5** | $0.293 \pm 0.085$ | $0.537 \pm 0.088$ | $0.750 \pm 0.135$ | $0.087 \pm 0.057$ | $0.108 \pm 0.038$ | $0.324 \pm 0.097$ |
| **6** | $0.267 \pm 0.107$ | $0.356 \pm 0.080$ | $0.800 \pm 0.144$ | $0.092 \pm 0.060$ | $0.174 \pm 0.061$ | $0.300 \pm 0.090$ |
| **average** | $0.240 \pm 0.072$ | $0.466 \pm 0.115$ | $0.699 \pm 0.107$ | $0.103 \pm 0.053$ | $0.152 \pm 0.053$ | $0.300 \pm 0.080$ |

TABLE S1: Tabulated $g$-factors plotted in Fig. S1. The average $g$-factor for each orientation is used in the main text to compare the anisotropy of the three QPCs.

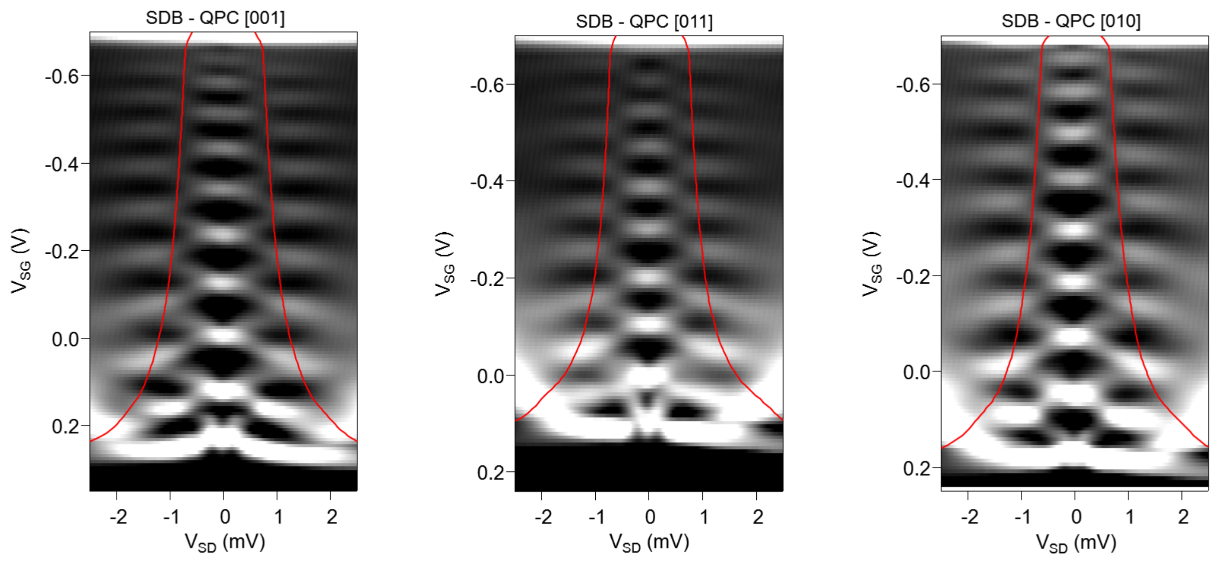


FIGURE S2: Grey-scale maps showing measured source-drain bias $V_{SD}$ for (a) QPC [001], (b) QPC [011], and (c) QPC [010]. Dark regions correspond to conductance plateaus, and white regions correspond to conductance risers or subband edges. The 1D subband energy spacings are are measured based on the quantity of dc bias applied to make adjacent subbands cross. For clarity the data shown here is 2-terminal, and the red overlaid lines indicate the series resistance correction to the dc bias.

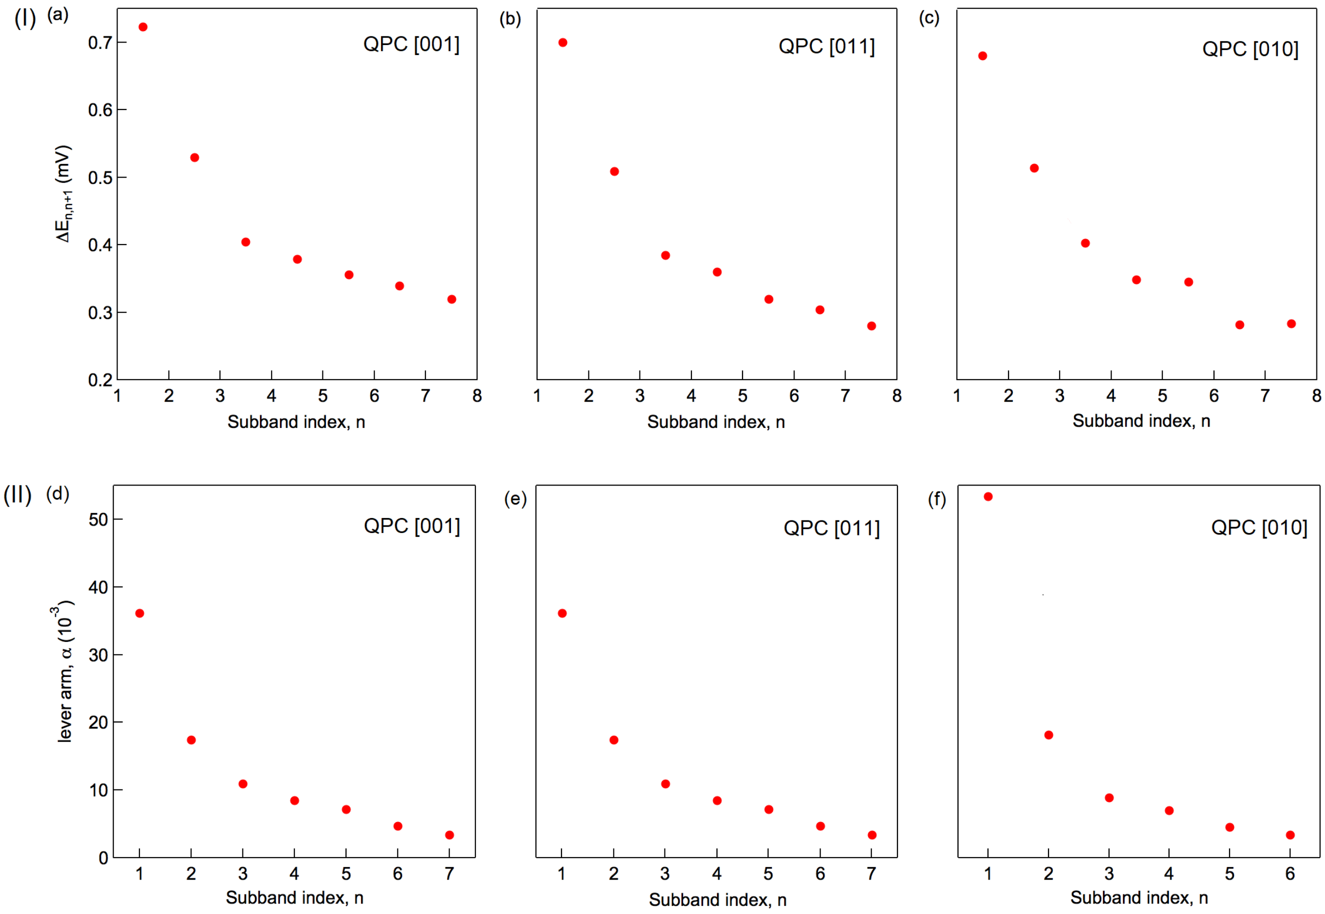


FIGURE S3: (I) 1D Subband spacing $\Delta E_{n,n+1}$ measured from the grey-scale source-drain bias maps in Supplementary Figure 2 for (a) QPC [001], (b) QPC [011], and (c) QPC [010]. (II) Lever-arm $\alpha$ for each subband for (d) QPC [001], (e) QPC [011], and (f) QPC [010].

| | $\gamma_1$ | $\gamma_2$ | $\gamma_3$ | $\kappa$ | $q$ | $\mathfrak{D}_1, meV\AA$ | $\mathfrak{D}_2, eV\AA^3$ | $\mathfrak{R}, \AA^2$ |
|---|---|---|---|---|---|---|---|---|
| Si | 4.29 | 0.34 | 1.45 | -0.42 | 0.01 | 0 | 0 | 0 |
| GaAs | 6.98 | 2.06 | 2.93 | 1.2 | 0.01 | 3.9 | 82 | 14.6 |
| InAs | 20.4 | 8.3 | 9.1 | 7.6 | 0.39 | 13 | 50 | 160 |
| InSb | 37.1 | 16.5 | 17.7 | 15.6 | 0.39 | 9.5 | 935 | 549 |

TABLE S2: Bulk parameters for Si, GaAs, InAs, InSb, see Ref. [1].

## II. NOTES ON THE THEORY

### A. 3D Hamiltonian

The effective 3D Hamiltonian that describes holes in cubic semiconductors in the long wavelength limit contains two parts: the Luttinger Hamiltonian that takes into account the general cubic symmetry of a crystal and the Dresselhaus Hamiltonian that results from the bulk inversion asymmetry in zinc-blende semiconductors:

$$H_{3D} = H_L + H_D, \tag{S2}$$

$$H_L = \left(\gamma_1 + \frac{5}{2}\gamma_2\right)\frac{\boldsymbol{p}^2}{2m} - \frac{\gamma_2}{m}\left(p_x^2 S_x^2 + \text{c.p.}\right) - \frac{\gamma_3}{2m}\left(\{p_x, p_y\}\{S_x, S_y\} + \text{c.p.}\right), \tag{S3}$$

$$H_D = \frac{\mathfrak{D}_1}{2}\left(p_x\{S_x, S_y^2 - S_z^2\} + \text{c.p.}\right) + \frac{\mathfrak{D}_2}{2}\left(S_x\{p_x, p_y^2 - p_z^2\} + \text{c.p.}\right) \tag{S4}$$

where $\boldsymbol{p}$ is the 3D hole momentum, $\boldsymbol{S}$ is the hole spin $S = 3/2$, $m$ is the bare electron mass, $\gamma_i$ are Luttinger parameters, $\mathfrak{D}_i$ are Dresselhaus parameters, $\{\dots\}$ is anticommutator, c.p. stands for cyclic permutations of indices $x$, $y$ and $z$. Cartesian components of the hole spin $\boldsymbol{S}$ and momentum $\boldsymbol{p}$ are written in main axes of the cubic crystal lattice: $X = [010]$, $Y = [001]$, $z = [100]$. The Hamiltonian $H_{3D}$ describes the spectrum of a free 3D hole in a cubic semiconductor.

In presence of electrostatic potential $V(x, y, z)$ one must add it to the Hamiltonian $H_{3D}$. As $H_{3D}$ does not include the conductance band, we have to account for the corresponding mixing of the conductance band through the derivatives of the potential which is referred to as the intrinsic Rashba spin-orbit interaction (SOI):

$$H_R = \mathfrak{R}\left[\boldsymbol{\nabla} V \times \boldsymbol{p}\right] \cdot \boldsymbol{S} \tag{S5}$$

where $\mathfrak{R}$ is the intrinsic Rashba parameter. There are also tensor contributions to $H_R$ but they are two orders of magnitude smaller than $H_R$ in GaAs. $H_R$ does not provide any original effect that stays apart of the usual Luttinger Hamiltonian, so we include this term only for completeness.

Apart of the electrostatic potential, we also apply the magnetic field $\boldsymbol{B}$ which can be included (i) through the long derivatives $\boldsymbol{p} \to \boldsymbol{p} - e\boldsymbol{A}$ in Eqs. (S2), (S3), (S4), (S5) where $\boldsymbol{A}$ is the vector-potential, or through (ii) Zeeman terms:

$$H_Z = -2\kappa\mu_B \boldsymbol{B} \cdot \boldsymbol{S} \tag{S6}$$

$$H_Z' = -2q\mu_B\left(B_x S_x^3 + c.p.\right) \tag{S7}$$

where $\kappa$ is the bulk hole $g$-factor, $q$ is the anisotropic hole $g$-factor. Even though $q \ll \kappa$ we still keep the $q$-term because we investigate the tensor effects here. All in all, the full 3D Hamiltonian we start from is the following:

$$H_{tot} = H_{3D} + V(x, y, z) + H_R + H_Z + H_Z' \tag{S8}$$

where we imply long derivatives in the momentum i.e. different components of the hole momentum do not commute.

The bulk parameters for Si, GaAs, InAs and InSb are given in Table S2.

## B. 2D effective Hamiltonian, B = 0

In this section we consider 2D heterostructure that can be modeled by some electrostatic potential $V(z)$. We only consider the case of (100) heterostructures i.e. the $z$-axis is directed along [100]. The electrostatic confinement $V(z)$ leads to 2D subbands where the ground subband originates from so-called heavy hole states with spin projections $S_z = \pm 3/2$. In absence of magnetic field the in-plane momentum is conserved, so we consider 2D plane waves. The spectrum of these plane waves can be described by effective 2D Hamiltonian that does not depend on the transverse $z$ degree of freedom. In order to avoid confusion, we use the notation $\boldsymbol{k} = (k_x, k_y) = (p_x, p_y)$ for in-plane components of the momentum.

As we include tensor corrections in the consideration, the dispersion is not axially symmetric. Tensor corrections carry non-zero components of angular momentum. For example, the Luttinger Hamiltonian can be expanded into axially symmetric part and the part $H_L^{tens}$ that carries projections of the total angular momentum $\pm 4$:

$$H_L^{tens} = \frac{\gamma_3 - \gamma_2}{8m}\left(k_+^2 S_+^2 + k_-^2 S_-^2\right) \tag{S9}$$

written in the crystal axes coordinate system $X = [010]$, $Y = [001]$, $Z = [100]$. After rotation of the coordinate system (which is by default the crystal axes system) by angle $\phi$ around the $z$-axis each vector component acquires the phase factor $e^{i\phi}$, e.g. $k_+ \to k_+ e^{i\phi}$. Therefore, the part $k_+^2 S_+^2$ acquires the factor $e^{4i\phi}$ in new coordinate system which corresponds to projection $j_z = +4$ of the total angular momentum. Therefore, our effective Hamiltonian must also contain terms that carry momenta $j_z = \pm 4N$, $N = 1, 2, \ldots$ if we couple $H_L^{tens}$ at least $N$ times through the perturbation theory. These terms, however, are suppressed by factor $\eta^N$ where

$$\eta = \frac{\gamma_3 - \gamma_2}{\gamma_3 + \gamma_2} \tag{S10}$$

For most semiconductors $\eta \ll 1$ and we can apply expansion over the angular momentum (see Table S2). Practically, we only account for zero and first orders in $\eta$ assuming the higher order terms to be small. This approach however is not justified in Si where $\eta \sim 1$, see Table S1. The Dresselhaus Hamiltonian only carries projections $j_z = \pm 2$. As Dresselhaus SOI is usually not stronger than the tensor Luttinger contribution $H_L^{tens}$, we only account for terms in the effective Hamiltonian that are linear in Dresselhaus constants $\mathfrak{D}_i$.

Therefore, the general form of the 2D effective Hamiltonian without magnetic field is the following:

$$\begin{aligned} H_{2D} &= E_1(k) + E_2(k)\left(k_+^4 + k_-^4\right) + iE_3(k)\left(k_+^2 - k_-^2\right) + \\ & i\alpha_1(k)\left(\Sigma_+ k_-^3 - \Sigma_- k_+^3\right) + i\alpha_2(k)\left(\Sigma_+ k_+ - \Sigma_- k_-\right) + \\ & i\alpha_3(k)\left(\Sigma_+ k_-^7 - \Sigma_- k_+^7\right) + \beta_1(k)\left(\Sigma_+ k_- + \Sigma_- k_+\right) + \\ & \beta_2(k)\left(\Sigma_+ k_-^5 + \Sigma_- k_+^5\right) \end{aligned} \tag{S11}$$

where all introduced functions $E_i(k)$, $\alpha_i(k)$ and $\beta_i(k)$ are real functions of $k = \sqrt{k_x^2 + k_y^2}$ that can be found from the exact diagonalization of the total 3D Hamiltonian $H_{tot}$, Eq. (S8). Cyclic components of pseudo-spin $\boldsymbol{\Sigma} = \boldsymbol{\sigma}/2$, $\boldsymbol{\sigma}$ are Pauli matrices, and 2D momentum $\boldsymbol{k}$ are written in the crystal axes coordinate system $X = [010]$, $Y = [001]$. $\Sigma_+$ carries angular momentum $j_z = +3$ as it mixes $S_z = \pm 3/2$ heavy hole states. Functions $E_i(k)$ are spinless, where $E_1(k)$ is the axial approximation of the hole dispersion, $E_2(k)$ and $E_3(k)$ describe the warping of hole dispersion due to the cubic lattice correction $H_L^{tens}$ and Dresselhaus SOI (S4) respectively, $E_2(k)$ is linear on the cubic lattice anisotropy $\eta$, see Eq. (S10), $E_3(k)$ is linear on Dresselhaus constants $\mathfrak{D}_{1,2}$. Functions $\alpha_i(k)$ describe 2D Rashba splitting of the hole dispersion due to structural inversion asymmetry. These terms violate spatial parity, therefore, they vanish in symmetric heterostructures $V(z) = V(-z)$. However, they appear in asymmetric heterostructures and may contribute up to 50% to the Fermi energy. The function $\alpha_1(k)$ is called cubic Rashba SOI. This is the main contribution that appears in the axial approximation. Functions $\alpha_2(k)$ and $\alpha_3(k)$ carry angular momentum $j_z = \pm 4$ and therefore they are proportional to small parameter $\eta$. Functions $\beta_i(k)$ originate from Dresselhaus term (S4).

Apart of time reversal, hermiticity and rotational properties, we used one more symmetry to construct the effective Hamiltonian $H_{2D}$. The reflection of axes [011] and [01$\bar{1}$] does not change the initial 3D Hamiltonian $H_{tot}$, see Eq. (S8). Therefore, the 2D effective Hamiltonian must be also invariant under these reflections. $H_{2D}$ is the angular momentum expansion of the 2D heavy hole dispersion. In Eq. (S11) we only account for $j_z = 0, \pm 2, \pm 4$ terms and skip all higher harmonics. $j_z = \pm 2$ terms originate from the Dresselhaus SOI, see Eq. (S4). $j_z = \pm 4$ terms are linear in $\eta$ and originate from the cubic lattice anisotropy term, see Eq. (S9).

## C. 2D Zeeman Hamiltonian

In this section we include in-plane magnetic field $\boldsymbol{B} = (B_x, B_y, 0)$ and construct possible 2D kinematic structures that are linear in $\boldsymbol{B}$. For numerical calculations we use the gauge $\boldsymbol{A} = (B_y(z - z_0), -B_x(z - z_0), 0)$ where constant $z_0$ is chosen in a way that $\boldsymbol{k} = 0$ corresponds to the minimum of hole dispersion, see discussion in Ref. [2]. Since the vector potential depends only on $z$, there are no vector-potential terms in 2D effective Hamiltonian. Applying the same symmetry consideration as in the previous section, we get the general form of the 2D Zeeman (linear in $\boldsymbol{B}$) Hamiltonian:

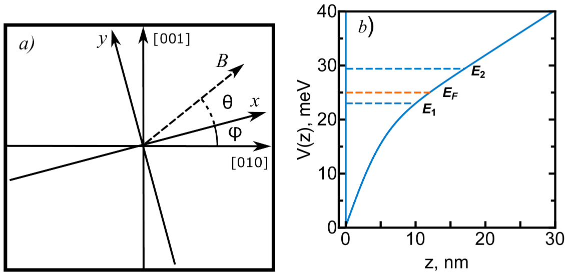


FIGURE S4: Panel a): Coordinate system $(x, y)$ used in Eq. (S12). $\boldsymbol{B}$ makes angle $\theta$ with the $x$-axis, the $x$ axis makes angle $\phi$ with [010] crystal axis. Panel b): Single heterojunction potential well $V(z)$ plotted with account of screening due to finite hole density in the leads $n = 2 \times 10^{11}\,\mathrm{cm}^{-2}$. $E_{1,2}$ correspond to bottoms of the ground and first excited 2D hole subbands, $E_F$ is the Fermi energy corresponding to the density $p = 2 \times 10^{11}\,\mathrm{cm}^{-2}$.

$$H_B = -\frac{g_1(k)}{2}\left(\Sigma_+ B_- k_-^2 + h.c.\right) - \frac{g_2(k)}{2}\left(\Sigma_+ B_+ k_-^4 + h.c.\right) - \frac{g_3(k)}{2}\left(\Sigma_+ B_+ e^{4i\phi} + h.c.\right) - \frac{g_4(k)}{2}\left(\Sigma_+ B_- k_+^2 e^{4i\phi} + h.c.\right) - \frac{g_5(k)}{2}\left(\Sigma_+ B_- k_-^6 e^{-4i\phi} + h.c.\right) - \frac{g_6(k)}{2}\left(\Sigma_+ B_+ k_-^8 e^{-4i\phi} + h.c.\right) - i\frac{g_{D1}(k)}{2}\left(\Sigma_+ B_- e^{2i\phi} - h.c.\right) - i\frac{g_{D2}(k)}{2}\left(\Sigma_+ B_+ k_-^2 e^{2i\phi} - h.c.\right) - i\frac{g_{D3}(k)}{2}\left(\Sigma_+ B_- k_-^4 e^{-2i\phi} - h.c.\right) - i\frac{g_{D4}(k)}{2}\left(\Sigma_+ B_+ k_-^6 e^{-2i\phi} - h.c.\right) + i\frac{\zeta_1(k)}{2}\left(B_+ k_- - h.c.\right) + i\frac{\zeta_2(k)}{2}\left(B_+ k_+^3 e^{4i\phi} - h.c.\right) + i\frac{\zeta_3(k)}{2}\left(B_+ k_-^5 e^{-4i\phi} - h.c.\right) - \frac{\zeta_{D1}}{2}\left(B_+ k_+ e^{2i\phi} + h.c.\right) - \frac{\zeta_{D2}}{2}\left(B_+ k_-^3 e^{-2i\phi} + h.c.\right) \tag{S12}$$

For simplicity we say that $\mu_B = 1$ and $k_\pm = (k_x \pm ik_y)/k$ in Eq. (S12) to make all couplings dimensionless, $h.c.$ stands for hermitian conjugate. Functions $g_i(k)$, $g_{Di}(k)$, $\zeta_i(k)$ are functions of $k = \sqrt{k_x^2 + k_y^2}$. $H_B$ is written in a coordinate system $(x, y)$ where $x$-axis makes angle $\phi$ with the crystal axis $X = [010]$. It leads to phase factors $e^{j_z i\phi}$ that explicitly indicate projection $j_z$ of the total angular momentum. Components $g_{1,2}(k)$ correspond to the axial approximation, see Ref. [2]. Terms $g_3(k)$, $g_4(k)$, $g_5(k)$, $g_6(k)$ carry angular momentum $j_z = \pm 4$ and therefore they are proportional to $\eta$. Terms $g_3(k)$ and $g_4(k)$ were calculated before in the limit of small in-plane momentum, see Refs. [2, 3]. Terms $g_{Di}(k)$ are proportional to the Dresselhaus constants $\mathfrak{D}_{1,2}$. Three $\zeta_i(k)$ terms are spinless and out of interest of the present work. Angular harmonics with $|j_z| \geq 6$ are neglected.

There is no need for such a pi/2 shift in the figures in main text because the Dresselhaus SOI is not included there i.e. the figures are pi/2 periodic.

Let us direct $/k$ along the $y$-axis, i.e. $k_+ = i$, $k_- = -i$, that makes angle $\phi$ with the crystal axis $X = [010]$, (we have already set $k_\pm = (k_x \pm ik_y)/k$ in Eq. (S12), see Fig. S4a. Magnetic field $\boldsymbol{B}$ makes angle $\theta$ with the x-axis which plays the role of the QPC axis, i.e. $B_\pm = Be^{\pm i\theta}$. Then, $H_B$ can be represented in the form

$$H_B = -\frac{B}{2}\left(\Sigma_+ M_+ + h.c.\right) - \frac{B}{2} M_0 \tag{S13}$$

where we introduced angular dependent magnetic moments

$$M_+ = -g_1 e^{-i\theta} + g_2 e^{i\theta} + (g_3 e^{i\theta} - g_4 e^{-i\theta})e^{4i\phi} + + (-g_5 e^{-i\theta} + g_6 e^{i\theta})e^{-4i\phi} + i(g_{D1} e^{-i\theta} - g_{D2} e^{i\theta})e^{2i\phi} + + i(g_{D3} e^{-i\theta} - g_{D4} e^{i\theta})e^{-2i\phi} \tag{S14}$$

$$M_0 = -2(\zeta_1 \cos(\theta) + \zeta_2 \cos(\theta + 4\phi) + \zeta_3 \cos(\theta - 4\phi)) + - 2(\zeta_{D1} \sin(\theta + 2\phi) + \zeta_{D2} \sin(\theta - 2\phi)) \tag{S15}$$

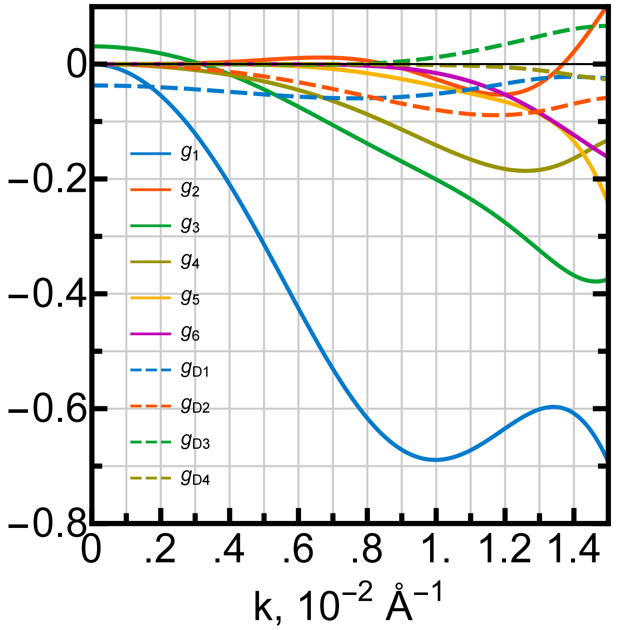


FIGURE S5: $g$-functions, see Eq. (S12), as functions of the in-plane momentum $k$. Units of $k$ are $10^{-2}$ Å$^{-1}$.

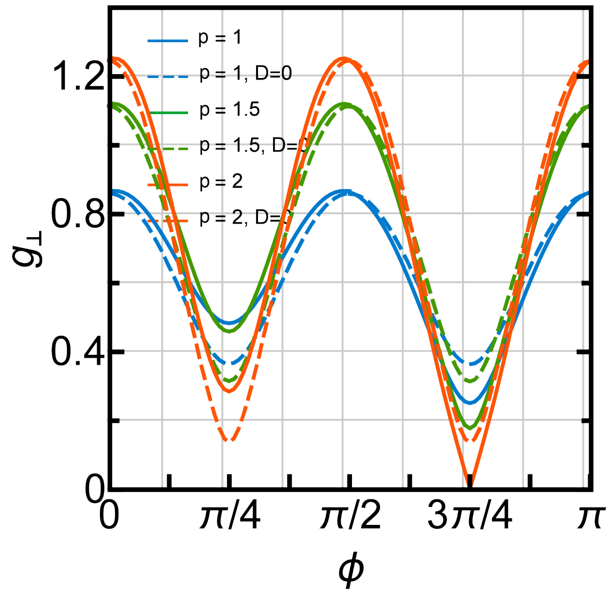


FIGURE S6: Perpendicular g-factor, see Eq. (S19), as function of $\phi$ for different densities: $p = 1$ (blue), $p = 1.5$ (green), $p = 2$ (red) in units $10^{11}$ cm$^{-2}$. Solid lines stand for the exact diagonalization, dashed lines stand for the effective Hamiltonian (S12).

$$\Delta E \cdot \Delta t \geq \frac{\hbar}{2} \tag{S16}$$

In other words the function $M_+$ that yields the spin splitting of 2D spectrum can be uniquely expanded via Fourier harmonics with different $j_z = j$:

$$M_+(\theta, \phi) = \sum_{j=-\infty}^{\infty} (g_j^+ e^{i\theta} + g_j^- e^{-i\theta}) e^{ij\phi} \tag{S17}$$

where $g_j^{\pm}$ correspond to different kinematic structures in the effective 2D Hamiltonian. In our case we only included $j = 0, \pm 2, \pm 4$, see Eq. (S17). Therefore, calculating numerically the function $M_+(\theta, \phi)$ and retrieving corresponding Fourier harmonics we construct the effective 2D Zeeman Hamiltonian for holes.

For numerical calculations we use the potential of single heterojunction (SHJ), see Fig. S4b, which is modeled for real device using NextNano software. Experimental density in the leads $p = 2 \times 10^{11}$ cm$^{-2}$ which corresponds to the Fermi energy $E_F \approx 2$ meV (above the ground subband edge $E_1$, see Fig. S4b). This Fermi energy is lower than the edge $E_2$ of first excited subband. Therefore, the effective Hamiltonian approach presented above is applicable to the device. Numerically calculated functions $g_i(k)$ and $g_{Di}(k)$ are plotted in Fig. S5. The Fermi momentum that corresponds to the density $p = 2 \times 10^{11}$ cm$^{-2}$ is $k_F = 1.12 \times 10^{-2}$ Å$^{-1}$. In this case $g_1$ is the dominant contribution, $g_3$ and $g_4$ are also important and they will result in huge $g$-factor anisotropy as function of angle $\phi$.

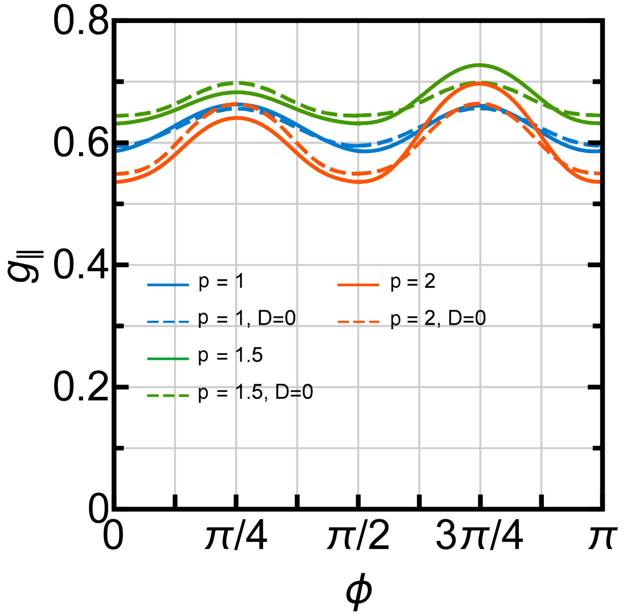


FIGURE S7: Parallel g-factor, see Eq. (S19), as function of $\phi$ at different densities: $p = 1$ (blue), $p = 1.5$ (green), $p = 2$ (red) in units $10^{11}$ cm$^{-2}$. Solid lines stand for the exact diagonalization, dashed lines stand for the effective Hamiltonian (S12).

Here we define $g$-factor as an absolute value of the magnetic moment $M_+$:

$$g(\theta,\phi) = |M_+(\theta,\phi)| \quad \text{(S18)}$$

Let us also introduce parallel and perpendicular $g$-factors as follows:

$$g_{\parallel}(\phi) = g(0,\phi), \quad g_{\perp}(\phi) = g(\pi/2,\phi) \quad \text{(S19)}$$

These two $g$-factors play role of parallel and perpendicular $g$-factors in quantum point contacts, see Ref. [2]. Plots of $g_{\perp}(\phi)$ and $g_{\parallel}(\phi)$ for different hole densities are shown in **Fig. S6** and **Fig. S7**, respectively. $g_{\parallel}$ changes insignificantly and can be well-approximated by simple axial model. However, $g_{\perp}$ changes drastically as function of $\phi$ having maxima at $\phi = 0, \pi/2$ and minima at $\phi = \pi/4, 3\pi/4$. Solid (dashed) lines in **Figs. S6, S7** correspond to exact diagonalization of the Hamiltonian Eq. (S8) (the effective 2D model Eq. (S12) without Dresselhaus SOI contributions). We see that the effective model containing only the terms $g_i(k)$, $6 \geq i \geq 1$, see Eq. (S12), without the Dresselhaus SOI and high angular momentum harmonics with $|j_z| \geq 6$ agrees very well with the exact diagonalization. This means that the main contribution to the crystal axis anisotropy of the in-plane hole $g$-factors comes predominantly from the first-order contribution of the cubic lattice asymmetry term Eq. (S9).

Notice that we can also extract the contribution of the Dresselhaus SOI by looking at the difference of $g_{\perp}$-factors for QPCs along [011] and [01$\bar{1}$] directions:

$$|g_{\perp}([011]) - g_{\perp}([01\bar{1}])| = 2|g_{D1} + g_{D2} - g_{D3} - g_{D4}| \quad \text{(S20)}$$

where the absolute values are taken from both sides. At $k = k_F = 1.12 \times 10^{-2}\,\text{Å}^{-1}$ this difference is approximately 0.3 which is not small and can be potentially measured. Unfortunately, the [01$\bar{1}$] QPC on our wafer was not functional and we cannot measure this difference on our device. However, measuring this difference could probe directly the Dresselhaus SOI effect on the Zeeman splitting.

Presented theory can be also applied to quasi-1D systems like quantum point contact (QPC). Let us direct the QPC channel along the $x$ axis, see Fig. S4. Source drain bias spectroscopy allows to extract Zeeman splitting of QPC 1D subband edges. In the limit of large subband number we can apply semi-classical approach and separate total wave function into transverse standing wave and the wave which is propagating along the channel. As we are interested in splitting of subband edges, we set the wave vector of propagating wave to zero, $k_x = 0$, meaning that the wavelength $\lambda_x$ of the propagating wave is much longer than the wavelength $\lambda_y$ of standing wave: $\lambda_x \gg \lambda_y$. Assuming the QPC channel to be a square well, we conclude that the energy of the highest filled subband is equal to Fermi energy $E_F$, therefore, $\langle k_y^2 \rangle \approx k_F^2$. Functions $g_{\parallel}(\phi)$ and $g_{\perp}(\phi)$ taken at $k = k_F$ yield parallel ($\boldsymbol{B}$ is parallel to the QPC channel) and perpendicular ($\boldsymbol{B}$ is parallel to the QPC channel) $g$-factors.


[1] R. Winkler, *Spin-Orbit Coupling Effects in Two-Dimensional Electron and Hole Systems*, Springer-Verlag, Berlin, Heidelberg, 2003.

[2] D. S. Miserev, A. Srinivasan, O. A. Tkachenko, V. A. Tkachenko, I. Farrer, D. A. Ritchie, A. R. Hamilton, O. P. Sushkov, Phys. Rev. Lett. **1**19, 116803 (2017).

[3] Y. Komijani, M. Csontos, I. Shorubalko, U. Zülicke, T. Ihn, K. Ensslin, D. Reuter and A. D. Wieck, *EPL* **102**, 3 (2013).

[4] G. Vionnet, O. P. Sushkov, Phys. Rev. Lett. **1**16, 126801 (2016)
